# Supplementary material for: Network-aware Recommendations in the Wild: Methodology, Realistic Evaluations, Experiments
Source: arXiv:2010.03183 source file (2020-10-06)
Supplement: Supplementary file 1 [file Appendix.tex]

\begin{algorithm}
\begin{algorithmic} [1]
\caption{\red{long version}\\BFS on YouTube Recommendations}\label{alg:recommendation}
\Statex {$Input: v, N, C, W_{BFS}, D_{BFS}, HistV(optional)$} 
\Statex \Comment ($r_{c,j}$ is the $j^{th}$ content in the related list of content $c$)
\State $R\gets \emptyset$ \Comment List of contents to recommend
\State $L\gets \emptyset$ \Comment List of explored contents
\State $S_{0}\gets \{v\}$
\For {$i=1;~i++;~i\leq D_{BFS}$}
	\State $S_{i}\gets \emptyset$ \Comment (set of contents at depth $i$)
	\For {$c\in S_{i-1}$} \Comment from the beginning of the list
		\For {$j=1;~j++;~j\leq W_{BFS}$}
			\If {$r_{c,j} \notin L$}
				\State $S_{i}.\red{append}(r_{c,j})$ 
				\State $L.\red{append}(r_{c,j})$
				\If{$c\in C$}
					\State $R.\red{append}(r_{c,j})$
					\If {$||R||=N$}					
						\State $return~~R$
					\EndIf
				\EndIf				
			\EndIf
		\EndFor
	\EndFor
\EndFor
%\State $i\gets 1$
%\For {$c\in L$}
%	\If {$i>N$}
%		\State $break$
%	\ElsIf{$c\in C$}
%		\State $R.\red{append}(c)$
%		\State $i\gets i+1$
%	\EndIf
%\EndFor
\While {$i\leq N$}
	\For {$c\in L\setminus R$}
		\State $R.\red{append}(c)$
		\State $i\gets i+1$
	\EndFor
\EndWhile
\State $return~~R$
\end{algorithmic}
\end{algorithm}
